# Supplementary material for: Urban Scene Diffusion through Semantic Occupancy Map
Source: arXiv:2403.11697 source file (2024-03-19)
Supplement: Supplementary file 1 [file supp.tex]

% \clearpage
\setcounter{page}{1}

\setcounter{figure}{0}
 
\setcounter{table}{0}
 
\setcounter{equation}{0}

\section{Experiment Detail}
\subsection{Occupancy Dataset}
We leverage semantic occupancy maps from the dataset referred to as occ3d~\cite{occ3d}, which has been collected from the nuScenes dataset. The training and validation sets comprise 700 and 150 scenes, respectively. We have observed that in certain scenes, the ego vehicle travels only a short distance, which results in sparsity within the collected occupancy maps. To remedy this, we selectively exclude those scenes from the training set where the driving distance of the ego car is less than 15 meters. Conversely, we maintain the integrity of the validation set, keeping all 150 original scenes intact.

\subsection{Implementation Details}
\paragraph{Architecture}
Our method contains training of three models, including the 3D VQVAE for semantic occupancy map, 3D U-Net for denoising diffusion process and an encoder embedding BEV map. For the 3D VQVAE we downsample the input data to 1/4 resolution with 2 residual block in each resolution. The size of codebook for the embedded vector is 2048. For the 3D U-Net, we adhere to the conventional U-Net architecture, implementing a resolution scale of 1, 2, and 4. Moreover, we incorporate attention blocks specifically at the resolution levels of 2 and 4. 
% For 2D VQVAE, it shares simliar structure with 3D VQVAE with codebook of size 1024 and downsample the input BEV map to 1/4 resolution.

\paragraph{Training and inference}
During the training process, the VQVAE for semantic occupancy maps and the VQVAE for BEV maps are both trained 40 epochs to get converged. For the training of diffusion model, we keep training the model 100 epochs to get converged. We adopt Adam as optimizer with learning rate of $2\times 10^{-6}$. During inference time, we utilize DDIM as our sampler and sample 100 steps when generating samples. We set the scale of classifier free guidance  as 5.0 for all the samples. The training process takes about 300 GPU hours  in total and the sampling takes about 2s on A5000.

\subsection{Scene Synthesis}
\begin{figure}
    \centering
    \includegraphics[width=1\linewidth]{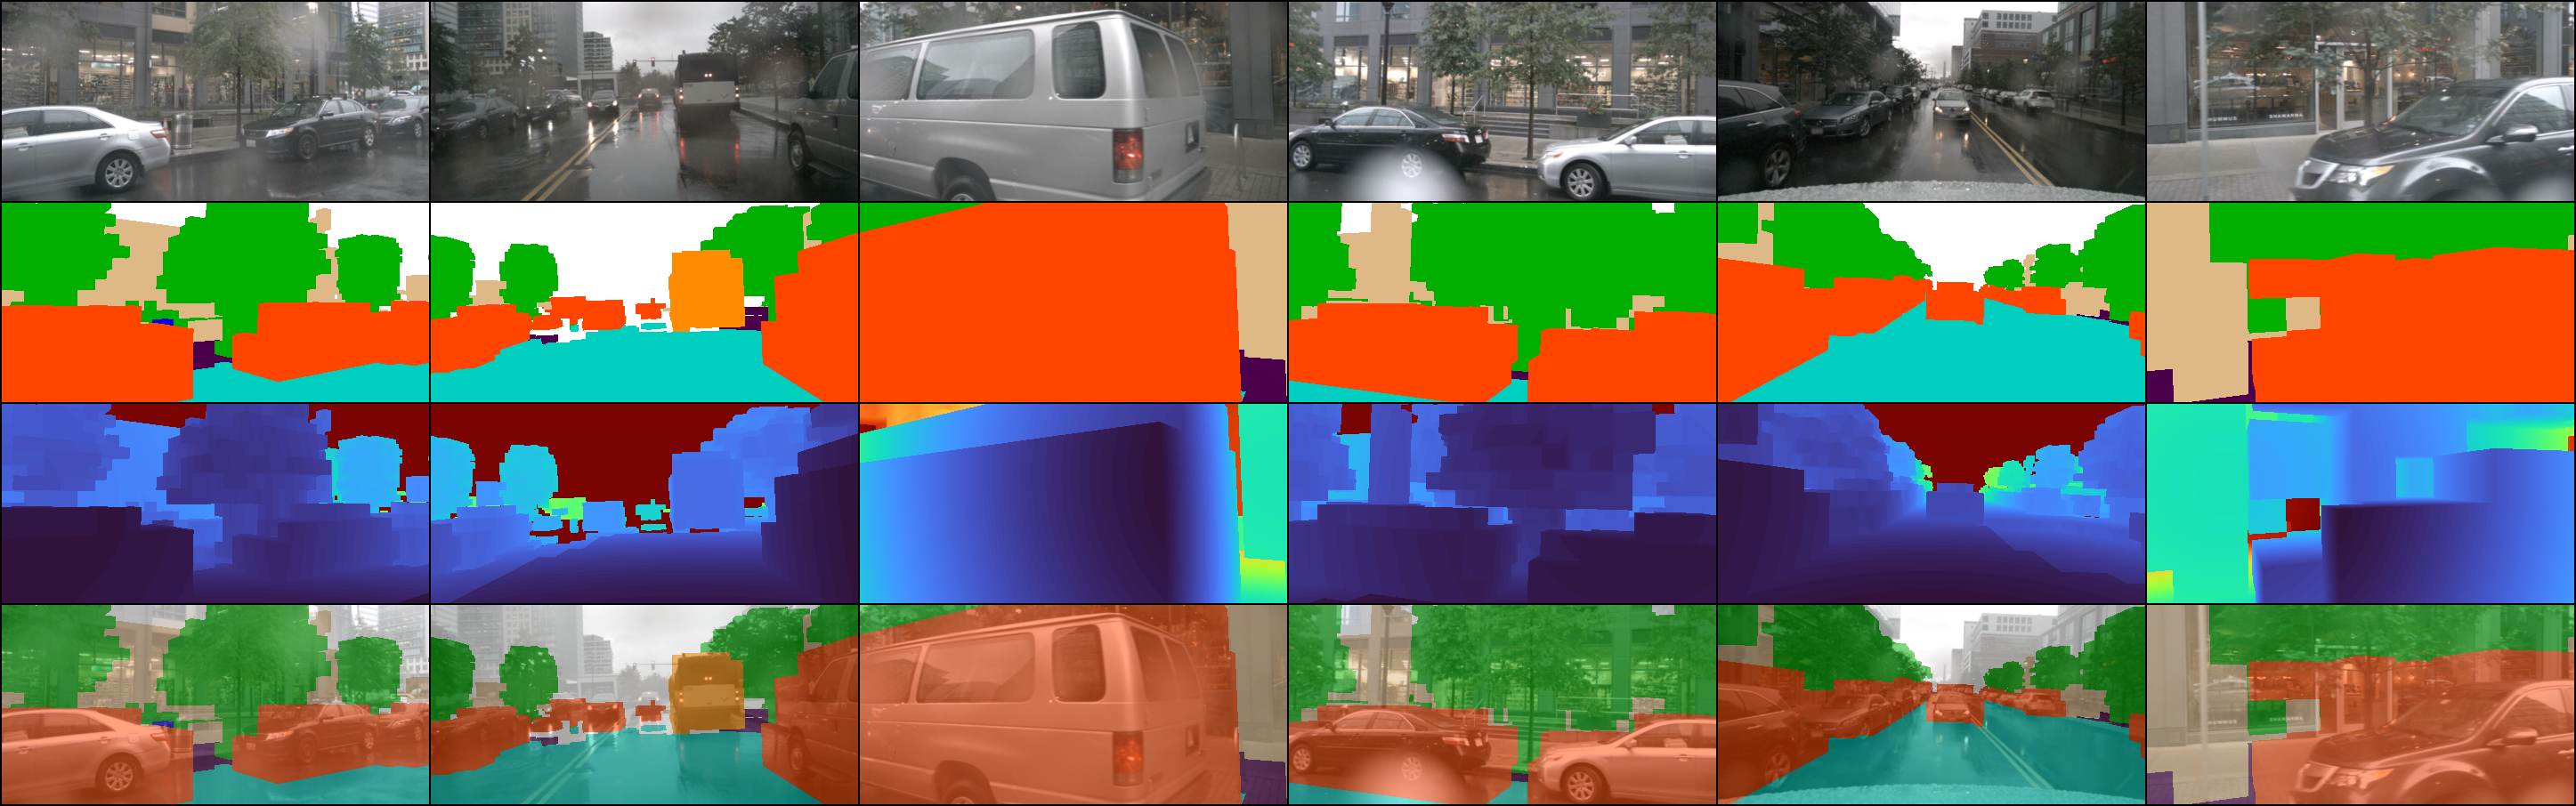}
    \caption{Visualization of the paired data from nuScenes dataset~\cite{nuscenes}. The second row and third row are 2D semantic map and depth map separately, which are projected from 3D semantic occupancy maps. The final row shows the combination of semantic map and rgb images.}
    \label{fig:pair_data}
\end{figure}
For scene synthesis, we fine-tune a 2D diffusion model~\cite{stablediff} via taking the paired data in Fig.~\ref{fig:pair_data} as conditional input through controlnet~\cite{controlnet}, and utilize the Score Distillation Sampling (SDS) ~\cite{dreamfusion} as prior to guide scene synthesis in our generated scenes. 

To be specific, we adopt the code base of threestudio\footnote{\url{https://github.com/threestudio-project/threestudio}} to implement the SDS guidance and utilize the 3D occupancy maps as occupancy grids to guidance the sampling of the volume rendering. For ray sampling, we sample 4 points in every grid which intersects with the sampled ray and sample 12 points per ray. We adopt a hash encoder with the resolution of 8192 and level dim of 8 to encode the coordinates of the sampled points.  For the background model, we adopt a hash grid encoder to model the background part, which only encodes the direction of rays. We optimize single-frame scenes which span 80 meters with 10,000 steps, and larger scenes which span 200 meters with 20,000 steps.

\subsection{More ablation studies}

We conduct ablation studies on guidance scale and ddim steps for detailed comparison. For SDS, we utilize it as an image prior to render the whole scenes so it cannot be replaced with other component to make comparison.
\begin{table}[ht!]
\centering
\setlength{\tabcolsep}{12pt}
\vspace{-3mm}
\resizebox{\linewidth}{!}{
\begin{tabular}{l|ccc|ccc}
\toprule
& \multicolumn{3}{c|}{Guidance scale} & \multicolumn{3}{c}{Inference steps} \\
& 2.5 & 5 & 10 & 50 & 100 & 150\\
\midrule
V-FID ($\downarrow$) & 275.2 & 291.4 & 302.1&295.6 & 291.4 & 290.2\\
MMD ($\downarrow$) &0.095 & 0.106 & 0.120& 0.110 & 0.106 & 0.103\\
\bottomrule
\end{tabular}
}
\caption{\textbf{Ablation for guidance scale and ddim steps.}}
\label{tab:ablation}
\vspace{-5mm}
\end{table}

\section{Metric}
\subsection{Quality metric}
To evaluate the quality of the generated samples, we embed the samples into feature space and further conduct scene evaluation with Fréchet Inception Distance(FID) \footnote{\url{https://github.com/mseitzer/pytorch-fid}} and Maximum Mean Discrepancy (MMD)\footnote{\url{https://github.com/yiftachbeer/mmd_loss_pytorch}}.

For the embedding process, we train a VQVAE to downsample the raw occupancy map to 1/8 resolution and the dimension of feature space is $24\times 24\times 2 \times 4$. The $24\times 24\times 2$ is the spatial dimension and 4 is the dimension of quantized vector. Then the feature vector would be flatten to a 1D vector with dimension of 4608 to calculate the FID and MMD.
\subsection{Consistency metric}
To evaluate the condition consistency between the generated samples and the input BEV map, we extract the data at ground level from the generated samples and compare the these data with the BEV label. All the labels in BEV which describe the attribute of road are merged into the road label. Consistency then could be calculated by evaluating the accuracy of the labels from generated samples.
\section{More qualitative results}
\paragraph{Scene Generation}
\begin{figure*}[ht!]
\centering

\includegraphics[width=1\linewidth]{fig/supp_fig_waymo_nuplan.pdf}

\vspace{-3mm}
\caption{Scenes generated from the BEV maps sampled from (a) the Waymo Motion Dataset\cite{waymo}  and (b) nuPlan Dataset~\cite{nuplan}. Even though our method do not utilize the data from waymo motion dataset and nuplan for training, we could also get reasonable scenes from these BEV maps.}
\label{fig:supp_fig}
\end{figure*}

We additionally test our method on the BEV map from Waymo Motion dataset~\cite{waymo} and nuPlan dataset~\cite{nuplan}. Our method could also generate reasonable samples from totally different BEV layout in Fig. ~\ref{fig:supp_fig}.
\paragraph{Scene Synthesis}
\begin{figure*}[ht!]
\centering

\includegraphics[width=1\linewidth]{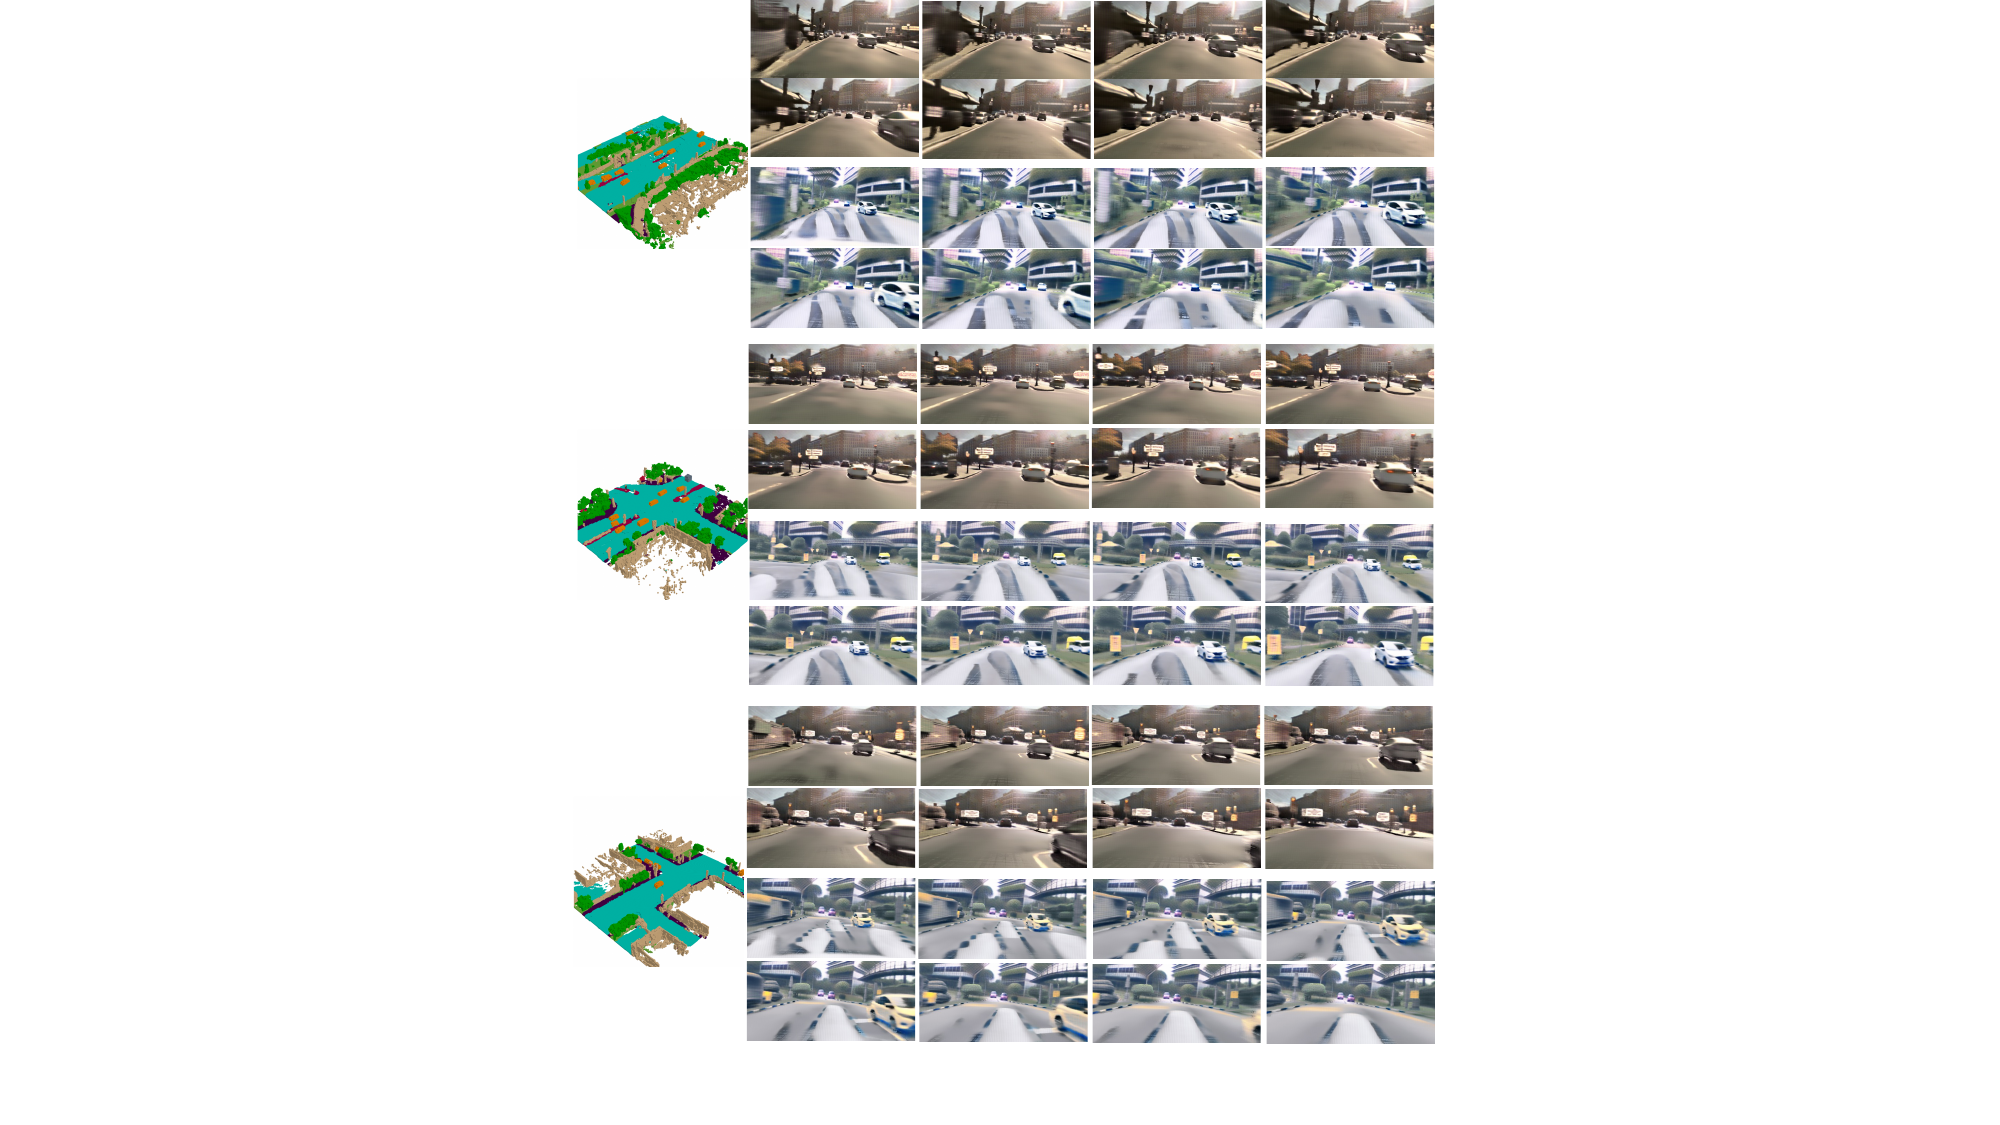}

\vspace{5mm}
\caption{Scenes synthesis on different generated samples. Our method ensures temporal consistency in the scene, thanks to the use of solid 3D representations. }
\label{fig:supp_fig_synthesis}
\end{figure*}

We perform scene synthesis on a variety of generated samples. As depicted in Fig.~\ref{fig:supp_fig_synthesis}, our method is capable of generating scenes with excellent temporal consistency. This demonstrates its potential for utilization as a simulation environment.

\paragraph{Video Demo}
We have included several video clips in our supplementary video materials. Please refer to these videos for a more comprehensive view of our qualitative results.
