# Supplementary material for: Urban Scene Diffusion through Semantic Occupancy Map
Source: arXiv:2403.11697 source file (2024-03-19)
Supplement: Supplementary file 2 [file supp_fig.tex]

\begin{figure*}[ht!]
\centering

\includegraphics[width=1\linewidth]{fig/supp_fig_waymo_nuplan.pdf}

\vspace{-3mm}
\caption{Scenes generated from the BEV maps sampled from (a) the Waymo Motion Dataset\cite{waymo}  and (b) nuPlan Dataset~\cite{nuplan}. Even though our method do not utilize the data from waymo motion dataset and nuplan for training, we could also get reasonable scenes from these BEV maps.}
\label{fig:supp_fig}
\end{figure*}
