# Supplementary material for: Urban Scene Diffusion through Semantic Occupancy Map
Source: arXiv:2403.11697 source file (2024-03-19)
Supplement: Supplementary file 3 [file supp_fig_synthesis.tex]

\begin{figure*}[ht!]
\centering

\includegraphics[width=1\linewidth]{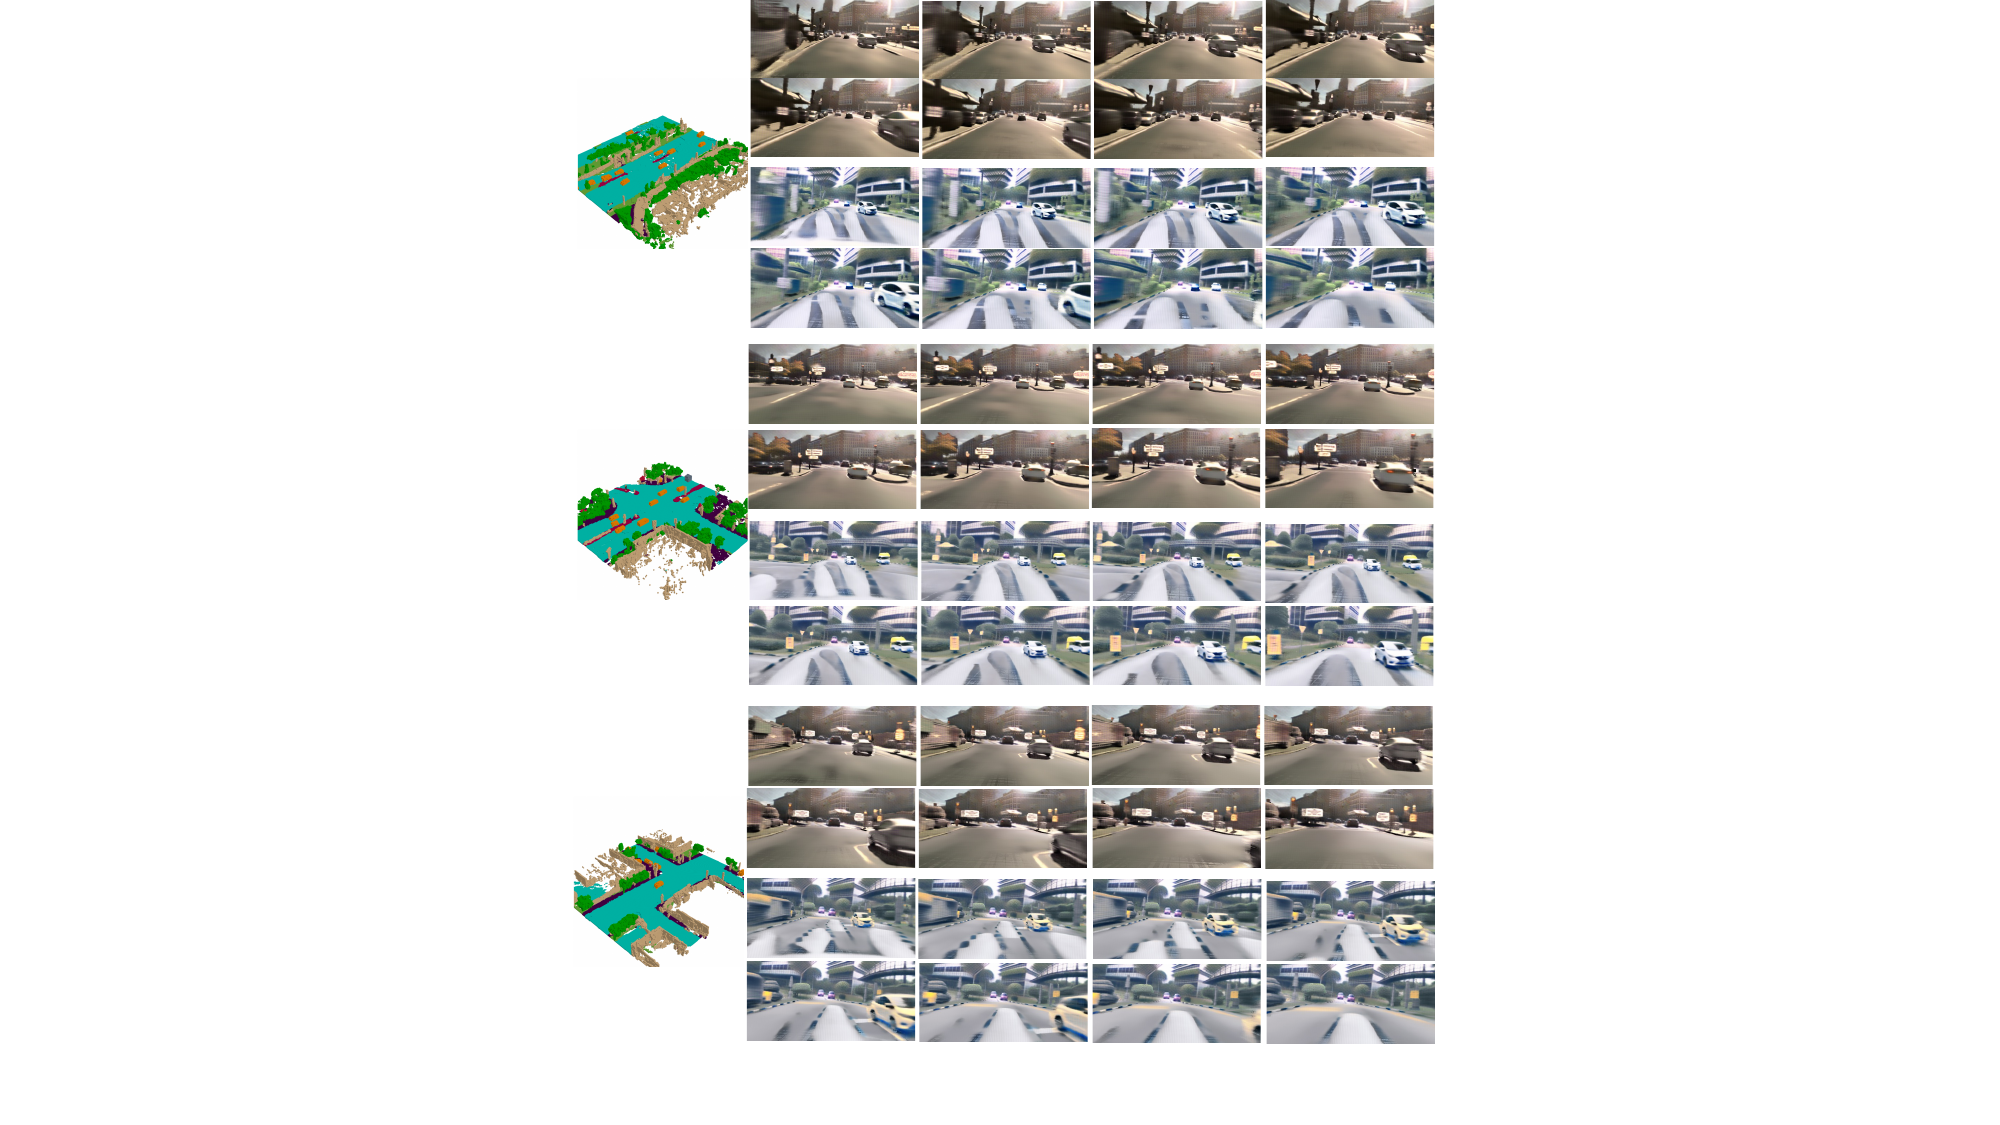}

\vspace{5mm}
\caption{Scenes synthesis on different generated samples. Our method ensures temporal consistency in the scene, thanks to the use of solid 3D representations. }
\label{fig:supp_fig_synthesis}
\end{figure*}
